# Supplementary material for: Conductance of graphene flakes contacted at their corners
Source: arXiv:1509.05261 ancillary file (2015-10-07)
Supplement: Supplementary file 1 [file SupplemInfo.pdf]

Supplementary Information (SI) to the paper

# Conductance of graphene flakes contacted at their corners

Martin Konôpka

Department of Physics,
Institute of Nuclear and Physical Engineering,
Faculty of Electrical Engineering and Information Technology,
Slovak University of Technology in Bratislava,
Ilkovičova 3, 812 19 Bratislava, Slovakia

7[th] October 2015

## 1 Armchair graphene nano-ribbons (AGNRs) with wide contacts to electrodes

We have recently considered AGNRs with wide contacts forming narrow strips [16] and also reviewed some of their stationary conductance properties (see also Appendix B therein). The results were obtained at zero gate voltage using the first NN TB approximation (1NNTBA). As a supplement to present work we consider the wide contacts again, now computing and plotting the linear conductance $G_{\rm lin}$ as a function of the gate voltage $V_{\rm g}$. We choose an AGNR of the width several times larger than its length (i.e. the size along the direction of the current flow), see inset of figure 1. This choice of the aspect ratio has been motivated by the knowledge that such short-wide AGNRs have been theoretically demonstrated [6, 7] to provide Ohmic-like electronic transport properties with theoretical conductivity $\sigma_{\rm dc} = (4/\pi)\, e^2/h = (2/\pi^2)\, e^2/\hbar$. This value has been obtained under the assumption that the electrodes are just smooth continuations of the AGNR. For our model of the electrodes we have obtained [16] a value denoted as $\sigma_{\rm wide} = 0.908\, \sigma_{\rm dc}$. We show our results for the conductance in figure 1, providing them for both the 1NNTBA (black dashed plot) and for

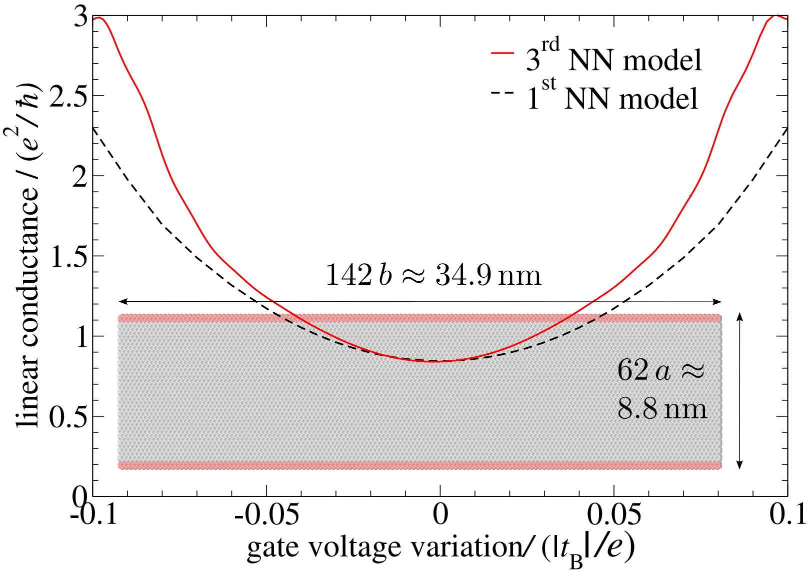


Figure 1: **Wide contacts:** The linear conductance is plotted as a function of the gate voltage for the armchair (ac) graphene nano-ribbon (AGNR) shown in the inset. Its size in terms of the number of atoms is 11 970. The red-colored strips on the AGNR margins mark the atoms to which the electrodes are coupled. (The armchair edges are oriented vertically on the image.) Each of the electrodes is 570 monoatomic wires thick. The results are obtained for the two different tight-binding approximations: the 1NNTBA (dashed black line) and the more accurate 3NNTBA (solid red line). The later curve has been horizontally shifted by $\Delta V_{\rm g} = +0.072\,|t_{\rm B}|/e$ (see the paper, section 2). We recall that $a \approx 1.42\,$nm is the NN distance in graphene and $b = a\sqrt{3} \approx 2.46\,$nm is the lattice parameter.

the more accurate third NN approximation (3NNTBA, solid red plot). The later curve has been horizontally shifted by $\Delta V_{\rm g} = +0.072\,|t_{\rm B}|/e$ so that its minimum approximately coincides with the minimum of the 1NNTBA plot. This is the same value of the shift as used for all $G_{\rm lin}$ plots computed by the 3NNTBA; see the comment in section 2 of the paper. The value $G_{\rm lin}(0) \approx 0.845\,e^2/\hbar$ yields $\sigma = (L/W)\,G_{\rm lin}(0) \approx 0.983\,\sigma_{\rm dc}$, a quantity similar to $0.908\,\sigma_{\rm dc}$ found in our referenced work; the minor difference may be due to different AGNRs used for the evaluation. Note that the above $\sigma_{\rm dc}$ is the theoretical value valid in the limit $W/L \gg 1$. The well-known feature of the 1NNTBA model is the symmetry of resulting dispersion relations, both for graphene and for the mono-atomically thin wires. The symmetry yields $G_{\rm lin}$ as an even function of the gate voltage: $G_{\rm lin}(V_{\rm g}) = G_{\rm lin}(-V_{\rm g})$. The dashed black plot utilises the symmetry: the values for negative $V_{\rm g}$'s have not been separately calculated. We have however verified using other example that our technique yields results precisely satisfying the $G_{\rm lin}(V_{\rm g})$ symmetry. The solid red plot (by the 3NNTBA) have been calculated in its whole range. After the application of the uniform $+0.072\,|t_{\rm B}|/e$ shift it acquires an almost symmetric shape. Results on figure 1 thus present a single minimum in the conductance, in agreement with the pioneering experimental work [5].

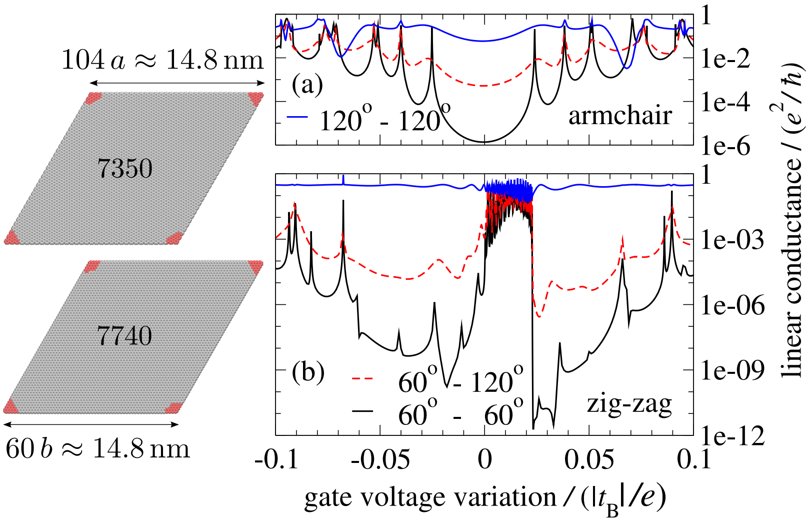


Figure 2: **Left panel:** graphical representation of two rhombic graphene flakes. The upper structure has the ac edges and uses electrodes 36 monoatomic wires thick. The lower structure has zig-zag (ZZ) edges and 35 monoatomic wires thick electrodes. See also descriptions to figures 2 and 3 in main text. **Right panel:** The linear conductance computed for the junctions formed by flakes shown on the left panel. **Graph (a):** the ac case. **Graph (b):** the ZZ case. The $60° - 60°$ plots (black solid lines) correspond to the case of both electrodes at the acute angles. Analogously the $120° - 120°$ plots (blue solid lines) describe the case of both electrodes at the obtuse angles. Finally the $60° - 120°$ plots (dashed red lines) present the mixed case. Legends like $120° - 120°$ apply globally within the whole figure.

## 2 Rhombus-shaped graphene flakes

As another supplement of our main work, we now turn our attention to junctions formed by flakes of rhombic form, with conductance computed using the 3NNTBA. Rhombi belong among prototypical structures providing both acute and obtuse angles. We investigate similar setups as we have done for the trapezoids in main text: (i) both electrodes at the acute (here 60°) angle corners: AA-AA setup, (ii) one electrode at the AA corner while the other attached at the obtuse angle corner: AA-OA setups, and finally (iii) both electrodes at the OA corners: OA-OA setup. While the trapezoidal flakes considered in main text provides the two different AA-OA combinations of the electrode pair attachments, rhombi allow only for a single one. Results for both ac and ZZ-edge terminated graphene sheets are shown in figure 2. We observe similar conductance characteristics as for the trapezoids and other structures studied in the present work.

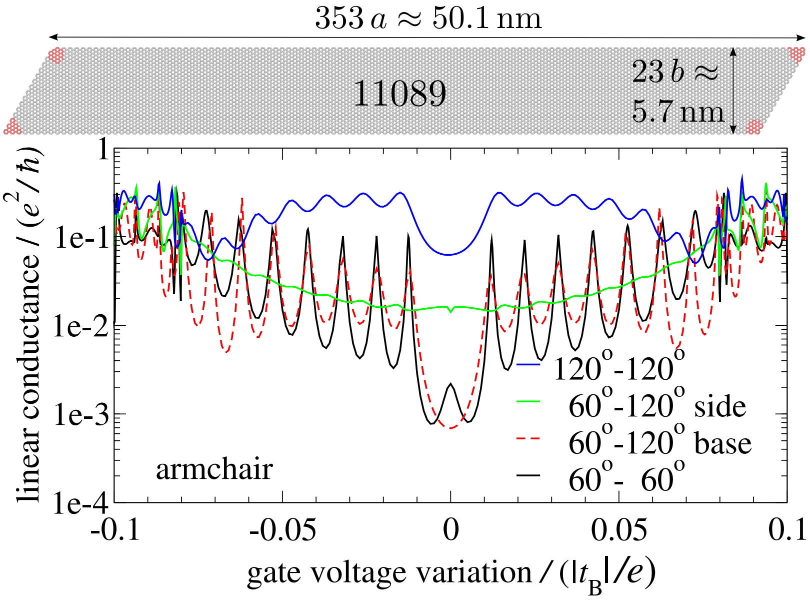


Figure 3: Similar kind of results like in figure 2 in main text or in figure 2 in this SI document but now the ac-edge terminated rhomboidal graphene flake is presented. The setup labelled as $60° - 120°$ *side* represents one electrode at the lower-left corner and the second electrode in the upper-left corner. Similarly the setup labelled as $60° - 120°$ *base* represents one electrode at the lower-left corner and the second one in lower-right corner. Each electrode is composed of 36 monoatomic wires.

# 3 Long-narrow rhomboids

Long-narrow rhomboidal graphene strips resemble ordinary long graphene nano-ribbons. They differ from them in corner angles which are 60° and 120° instead of just 90°. We perform analysis of their conductance similarly as for other structures within the present work. The results are shown within figures 3 and 4. The numbers of composing carbon atoms are also shown there: 11 089 for the ac case and 11 478 for the ZZ one. The dimensions of the rhomboidal ribbons are shown as well. The lengths and widths are chosen to be the same as those of the trapezoids corresponding to panels (d) of figures 2 and 3 in main text, respectively. We notify the reader that the two OA corners of the ac-edge terminated rhomboid on the figure have slightly different shapes, a sharp one on the right-hand side *vs.* a blunt one. The results shown in figures 3 and 4 confirm main findings of the present work, i.e. the contrast between the conductances in the AA-AA and OA-OA attachments. As expected, the rhomboid with the ZZ edges exhibits the $0.025\,|t_{\mathrm{B}}|$ narrow high-conductance window and otherwise the contrast between the AA-AA and OA-OA attachments is found again [figure 4]. Contrary to the results for the long-narrow ac-edge terminated trapezoid [figure 2(d) in main text], in case of the rhomboid the two different AA-OA setups are dissimilar (dashed green *vs.* solid red plot on figure 3). Instead, we observe similarity between the solid black

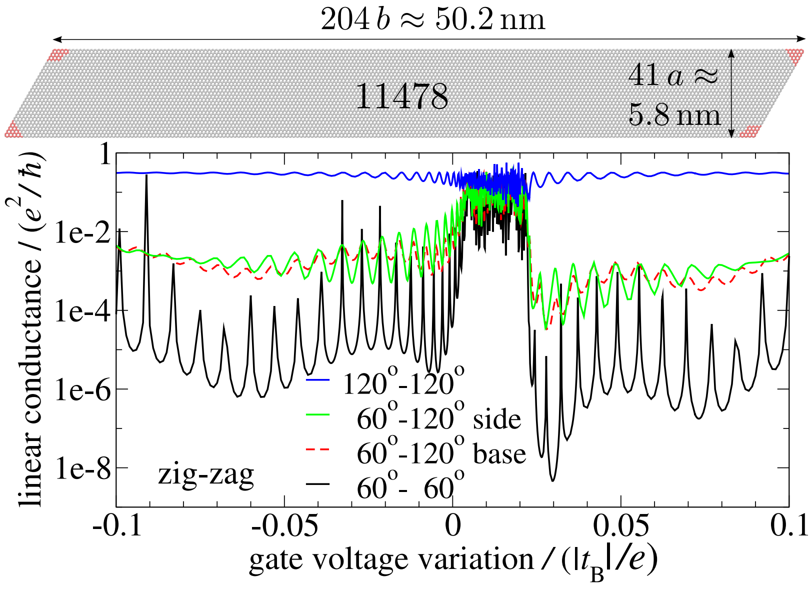


Figure 4: Results for ZZ-edge terminated rhomboid. Each electrode is now composed of 36 monoatomic wires. See caption to figure 3 for the rest of the description.

and dashed red plots. We do not analyse these features in detail and can at least say that the results are not completely counterintuitive. For instance, according our intuition, the dashed-red plot in figures 2(d) in main text should be similar to solid green plot in figure 3. The similarity is really found to be very close. In case of ZZ-edge terminated rhomboid we still find the quite close close proximity of the $G_{\mathrm{lin}}$ plots for the two different AA-OA setups (dashed red and solid green plots on figure 4). The same feature was found also in main text for the ZZ-edge terminated trapezoids, see figure 3(a,b,d) in main text and the text at the end of section 3.2 therein.

# 4 Long-narrow rhomboids in the 1$^{\mathrm{st}}$ NN approximation

Results obtained within the 1NNTBA, although being less accurate, are sometime more instructive and may help explanation of and presentation of more accurate results. For this reason we provide conductances of the long-narrow rhomboids computed now using the 1NNTBA (figures 5 and 6). They should be compared to results shown in the section 3 of this SI document. Note that data obtained within the 1NNTBA have not been post-processed by any $\Delta V_{\mathrm{g}}$ shift (explained in section 2 in main text) and the $G_{\mathrm{lin}}(V_{\mathrm{g}})$ functions from the 1NNTBA model would always be perfectly symmetric with respect to the Fermi level.

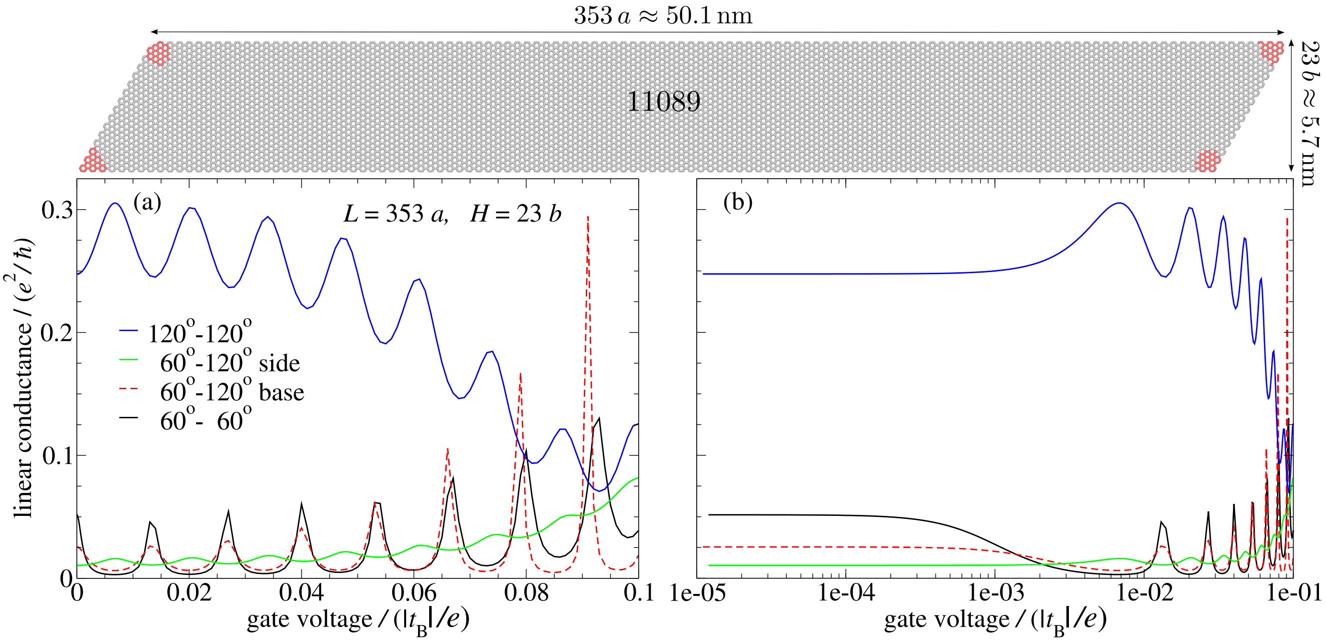


Figure 5: Results for the same system as presented in figure 3 but now obtained within the 1NNTBA model. Contrary to previous figures, here we opt for the linear scale on the vertical axes. Graphs (a) and (b) display identical sets of results, differing only by the scales used for the horizontal axes. Captions to figures 3 in this SI and in figure 2 in main text explain legends and colors used.

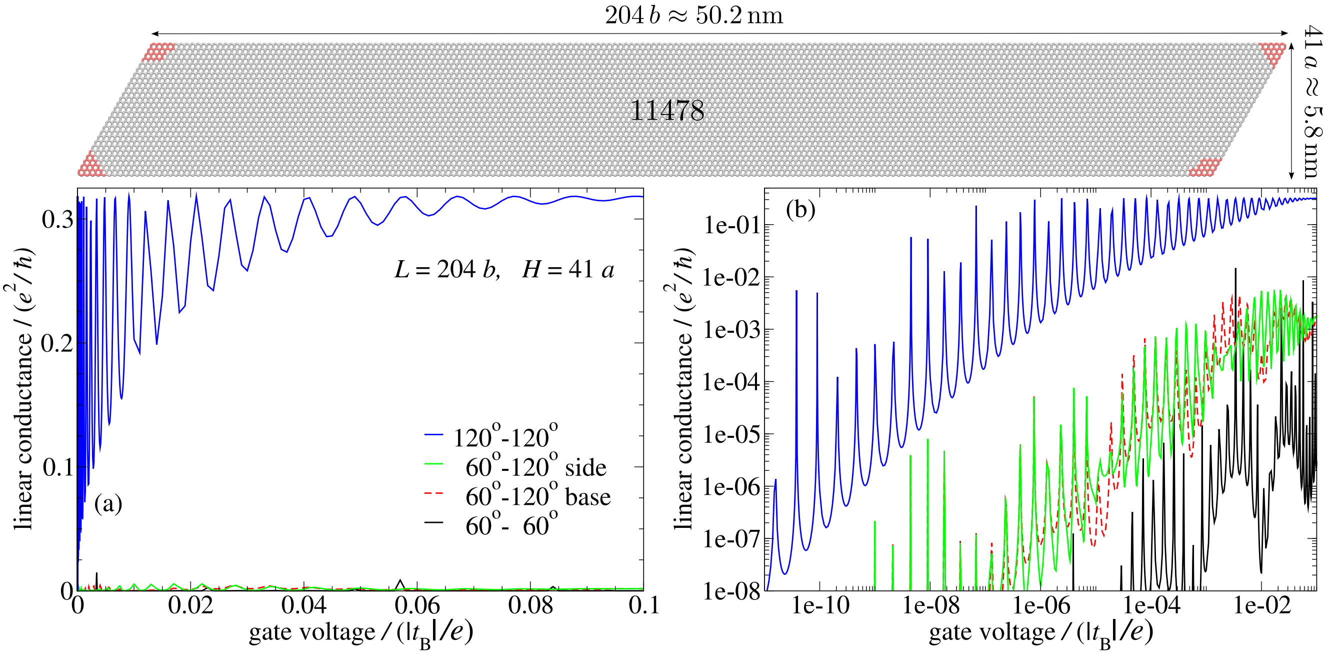


Figure 6: Results for the same system as presented in figure 4 but now obtained within the 1NNTBA model. Graphs (a) and (b) display identical sets of results. Graph (a) uses the linear scales on its both axes while graph (b) has both its axes scaled logarithmically.

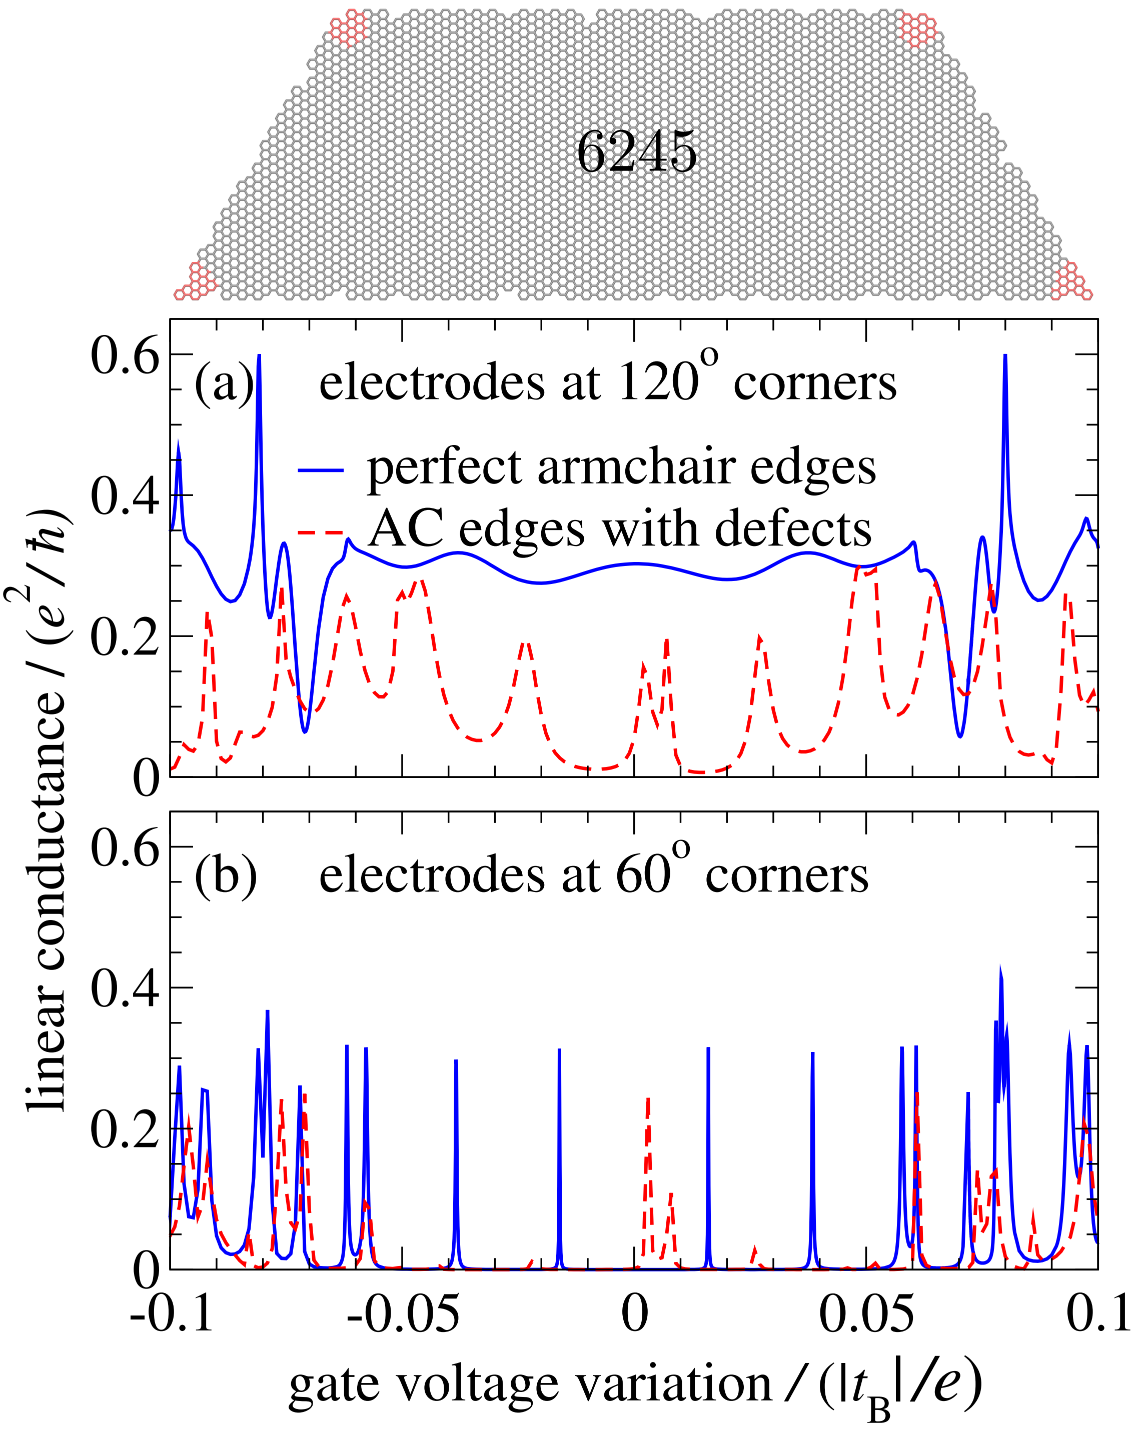


Figure 7: **Upper panel:** Graphical representation of the ac flake with the edge defects which is described in appendix C of the paper. It is based on the ac-edge terminated trapezoid shown in the left panel of figure 2 of the paper, the second structure from the top. See the paper for additional description. **Graph (a):** Direct comparison of the linear conductances of the junctions formed by the trapezoidal flake with perfect ac edges (solid blue curve) and by the flake with defects shown in the upper panel (dashed red curve). The electrodes are connected to the 120° angle corners. **Graph (b):** Analogous plots as in the graph (a) but now for the electrodes connected to the 60° angle corners.

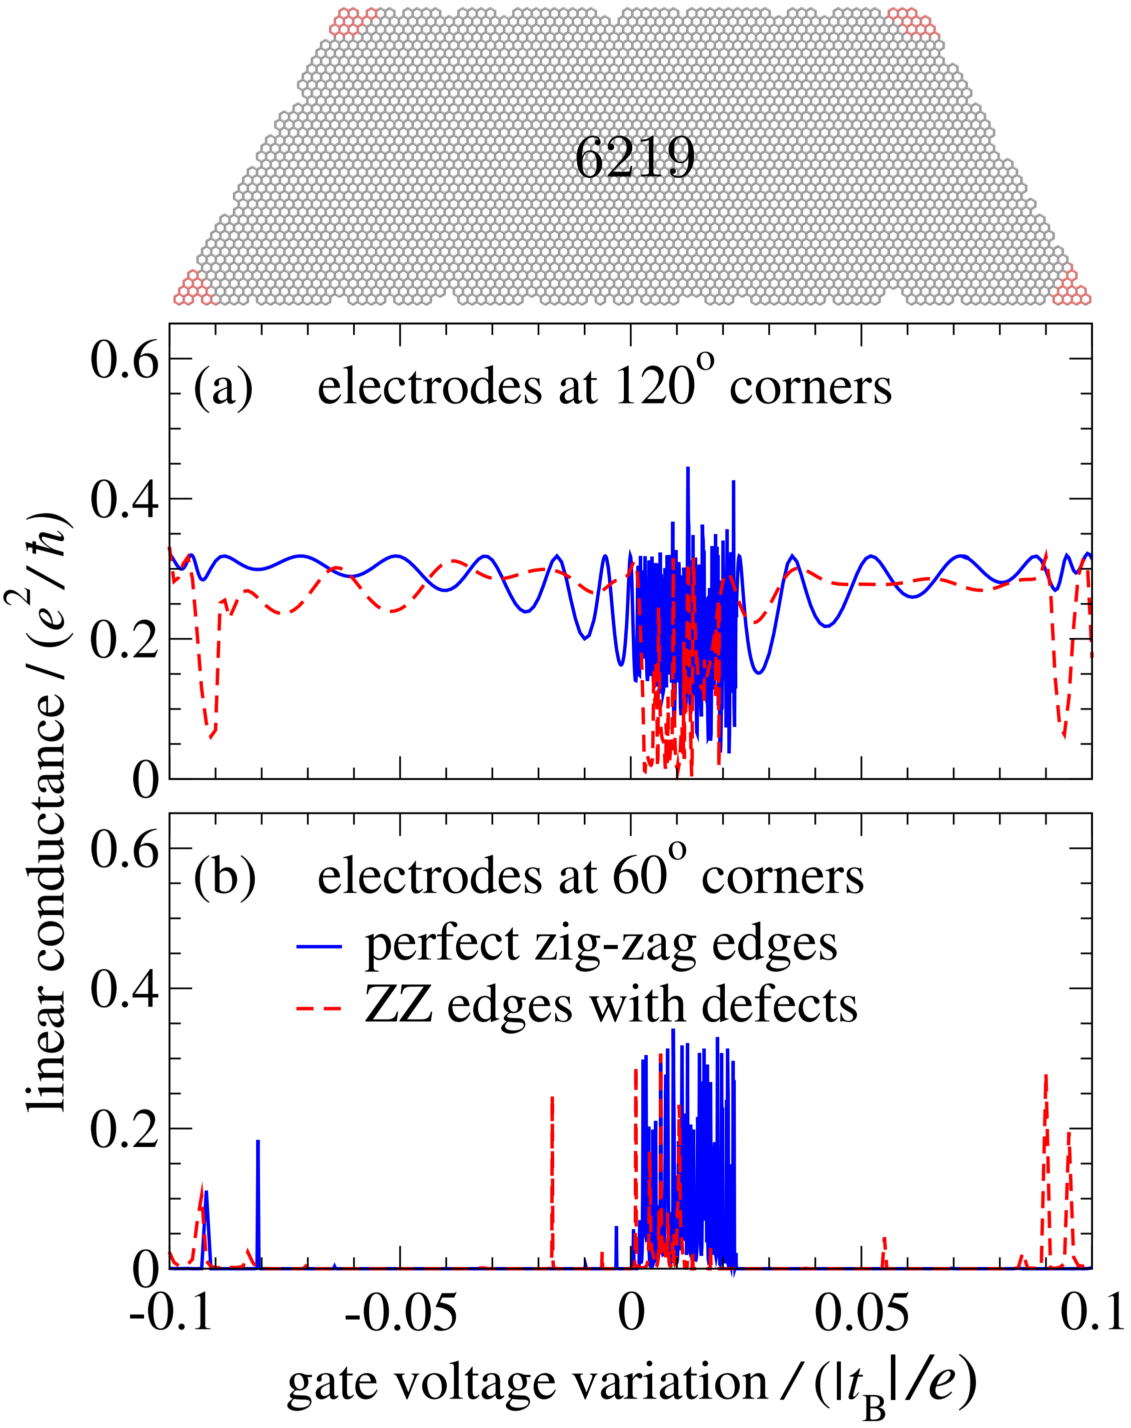


Figure 8: Upper panel: Graphical representation of the ZZ flake with the edge defects which is described in appendix C of the paper. It is based on the ZZ-edge terminated trapezoid shown in the left panel of figure 3 of the paper, the second structure from the top. The rest of the caption is the same or analogous as in figure 7 above.

## 5 Impact of the edge disorder

Within this section we show graphical representations of the two samples with irregular edges examined in appendix C of the paper (upper panels of figures 7 and 8). We also provide alternative presentations of the data shown in figures 13 and 14 of the paper, now displaying the conductance axes in linear scales and combining the data in order to provide direct comparisons between the cases of perfect and imperfect edges [graphs (a) and (b) in figures 7 and 8].

## References


[1] P.R. Wallace, *Phys. Rev.* **71**, 622 (1947).

[2] A.H. Castro Neto, F. Guinea, N.M.R. Peres, K.S. Novoselov and A.K. Geim, *Rev. Mod. Phys.* **81**, 109 (2009).

[3] K. Nakada, M. Fujita, G. Dresselhaus and M.S. Dresselhaus, *Phys. Rev. B* **54**, 17954 (1996).

[4] Y.-W. Son, M.L. Cohen and S.G. Louie, *Phys. Rev. Lett.* **97**, 216803 (2006).

[5] K.S. Novoselov, A.K. Geim, S.V. Morozov, D. Jiang, M.I. Katsnelson, I.V. Grigorieva, S.V. Dubonos and A.A. Firsov, *Nature* **438**, 197 (2005).

[6] M.I. Katsnelson, *Eur. Phys. J. B.* **51**, 157 (2006).

[7] J. Tworzydło, B. Trauzettel, M. Titov, A. Rycerz and C.W.J. Beenakker, *Phys. Rev. Lett.* **96**, 246802 (2006).

[8] N.T. Cuong, M. Otani and S. Okada, *Phys. Rev. B* **87**, 045424 (2013).

[9] M.F. Borunda, H. Hennig and Eric J. Heller, *Phys. Rev. B* **88**,125415 (2013).

[10] M. Settnes, S.R. Power, D.H. Petersen and A.-P. Jauho, *Phys. Rev. Lett.* **112** 096801 (2014).

[11] S. Reich, J. Maultzsch, C. Thomsen and P. Ordejón, *Phys. Rev. B* **66**, 035412 (2002).

[12] D.A. Areshkin, D. Gunlycke and C.T. White, *Nano Lett.* **7**, 204 (2007).

[13] L. Malysheva and A. Onipko, *Phys. Rev. Lett.* **100**, 186806 (2008).

[14] E. Perfetto, G. Stefanucci and M. Cini, *Phys. Rev. B* **82**, 035446 (2010).

[15] T. Ando, *J. Phys. Soc. Jpn.* **74**, 777 (2005).

[16] M. Konôpka and P. Bokes, *Phys. Rev. B* **89**, 125424 (2014).

[17] M. Lewkowicz and B. Rosenstein, Phys. Rev. Lett. **102**, 106802 (2009).

[18] D.A. Ryndyk, B. Song, R. Gutiérrez and G. Cuniberti, *Green Function Techniques in the Treatment of Quantum Transport at the Molecular Scale*, in *Energy Transfer Dynamics in Biomaterial Systems, edited by I. Burghardt, V. May, D.A. Micha and E. Bittner*, Springer Series in Chemical Physics Vol. 93 (Springer-Verlag, Berlin, Heidelberg, 2009), p. 213.

[19] M. Konôpka and P. Bokes, *Eur. Phys. J. B.* **86**, 114 (2013).

[20] E.R. Mucciolo, A.H. Castro Neto and C.H. Lewenkopf, *Phys. Rev. B* **79**, 075407 (2009).

[21] J. Li, I. Martin, M. Büttiker and A.F. Morpurgo, *Nat. Phys.* **7**, 38 (2011).

[22] W. Humphrey, A. Dalke and K. Schulten, *J. Molec. Graphics* **14**, 33 (1996).
